# Supplementary material for: Arbitrarily accurate representation of atomistic dynamics via Markov Renewal Processes
Source: arXiv:2008.11623 ancillary file (2020-08-26)
Supplement: Supplementary file 1 [file supporting-material.pdf]

# Supplementary materials

**Arbitrary accurate representation of atomistic dynamics via Markov Renewal Processes**
Animesh Agarwal, Sandrasegaram Gnanakaran, Nicholas Hengartner, Arthur F. Voter and Danny Perez
Theoretical Division, Los Alamos National Laboratory

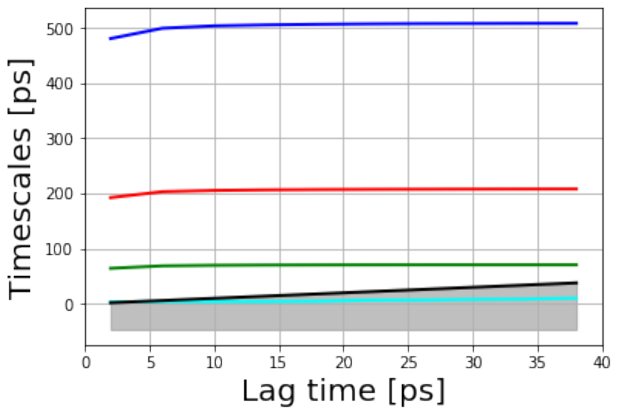


Figure 1: Implied timescale analysis of the alanine dipeptide simulations.

**Alanine Dipeptide Simulations:**

The simulation system comprises one alanine dipeptide molecule surrounded by 641 CHARMM TIP3P [1] water molecules. The molecular interactions between the different molecules are described by the CHARMM27 force field [2]. The simulation box is cube with length = 2.7 nm. We use AMBER molecular dynamics package to perform all the simulations using a timestep of 2 fs. We first perform a steepest-descent minimization and then perform equilibrium NPT simulation for 100ns. The temperature was fixed at 300 K by using a Langevin thermostat with friction coefficient 1.0 1/ps and the pressure was fixed using a Berendsen barostat with a pressure coupling constant of 4 ps. Finally, we perform a 2 μs long NPT production run using the same parameters for the thermostat and barostat. To model the Van der Waals interactions, we employ Lennard Jones potential with a cut-off radius of 1.2 nm. We employ the Particle Mesh Ewald (PME) [3] method for computing the electrostatic interactions. The cutoff for the direct space part of the PME was the same as that of Van der Waals interaction.

**MSM construction and analysis:**

In this work, we use the PyEMMA software package [4] for MSM construction and analysis. In the case of alanine dipeptide, we discretize the dihedral angle space using a 20x20 uniform grid. We compute the relaxation timescales as a function of lag time (shown in Figure 1) and observe a large spectral gap between the third and the fourth relaxation timescales, which suggests the presence of four metastable states. We then employ PCCA to obtain “crisp” state boundaries corresponding to the four metastable states, which can be seen in Figure 2. For the case of Chignolin, we employ time-lagged independent component analysis (TICA) [5] at a lag time of 50 ns to obtain the two slowest reaction coordinates using the backbone and side chain torsion angles in the protein as a feature set.

We discretize this space using a 25x25 uniform grid. We perform the implied timescales analysis (shown in Figure 3) and observe a large timescale separation between the first and the second relaxation timescale, indicating the presence of two metastable states. We therefore generate two metastable states using PCCA, which can be seen in Figure 4.

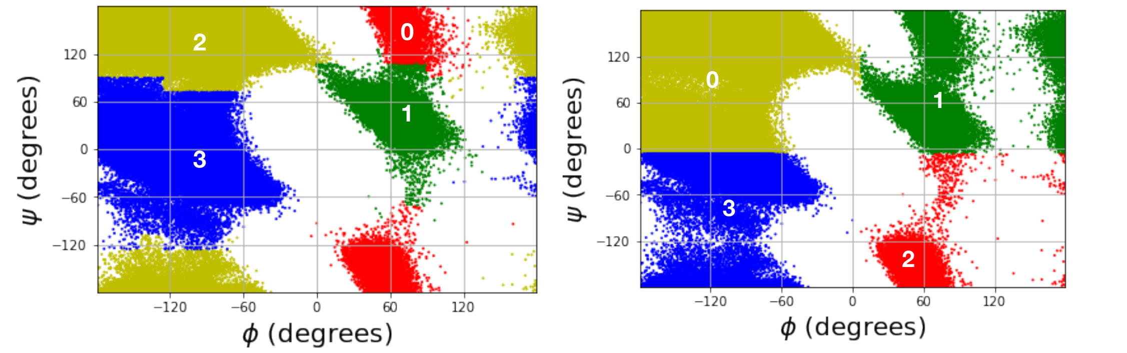


Figure 2: State definition for alanine dipeptide. Left: PCCA; Right: arbitrary.

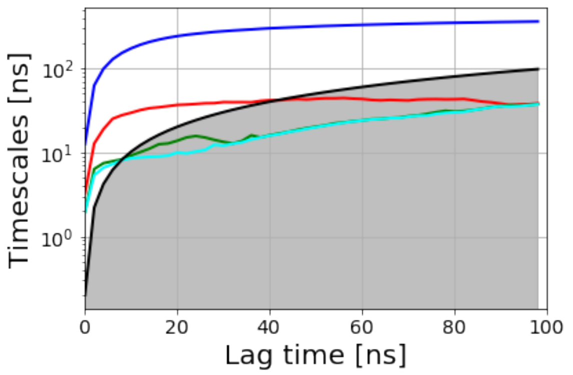


Figure 3: Implied timescale analysis of the chignolin simulations.

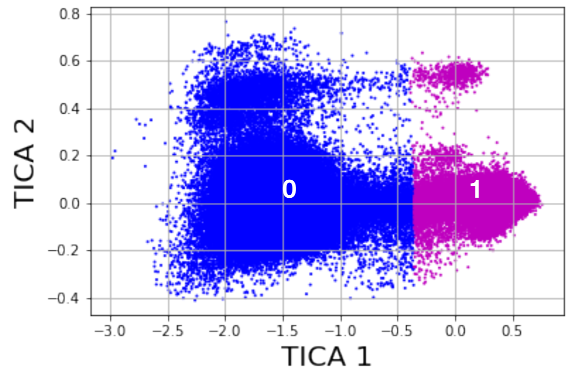


Figure 4: PCCA state definition for chignolin.

## References


1. W. L. Jorgensen, J. Chandrasekhar, J.D. Madura, R.W. Impey, and M.L. Klein., J. Chem. Phys., 79(2), 926 (1983).
2. N. Foloppe and A.D. MacKerell Jr., J. Comput. Chem., 21(2), 86 (2000)
3. T. Darden, D. York, and L. Pedersen, J. Chem. Phys., 98, 10089 (1993)
4. M.K. Scherer, B. Trendelkamp-Schroer, F. Paul, G. Perez-Hernandez, M. Hoffmann, N. Plattner, C. Wehmeyer, J.H. Prinz, and F. Noe, J. Chem. Theory Comput. 11, 5525 (2015)
5. G. Perez-Hernandez, F. Paul, T. Giorgino, G. De Fabritiis and F. Noe, J. Chem. Phys., 139, 015102 (2013)
